# Supplementary material for: API-BLEND: A Comprehensive Corpora for Training and Benchmarking API LLMs
Source: arXiv:2402.15491 source file (2024-05-20)
Supplement: Supplementary file 1 [file appendix.tex]

\section{Data flow diagram for SeqTopV2 creation}
Figure \ref{topv2_ex} represents an illustrative example of how the data has been curated from a semantic parsing dataset - SeqTopV2. 
 
\section{Input/Output Examples for Curated Datasets}
Below are some examples from different in-distribution datasets. 
\begin{nolinenumbers}
\begin{lstlisting}[language=json,firstnumber=1]
### SeqATIS ###
{
 "input": "could you please give me a one way fare from pittsburgh to atlanta , what airlines service pittsburgh airport and then houston airports",
 "output": "atis_airfare(round_trip = \"one way\"; fromloc.city_name = \"pittsburgh\"; toloc.city_name = \"atlanta\") [SEP] atis_airline(airport_name = \"pittsburgh airport\") [SEP] atis_airport(city_name = \"houston\")"
}

### SeqSGD ###
{
 "input": "Find a dentist in Sunnyvale named Amazing Smile Dental. Book an appointment at Amazing Smile Dental in Sunnyvale on March 10th at 1 pm.",
 "output": "FindProvider(city = \"Sunnyvale\"; dentist_name = \"Amazing Smile Dental\") [SEP] BookAppointment(appointment_date = \"March 10th\"; appointment_time = \"1 pm\"; city = \"Sunnyvale\"; dentist_name = \"Amazing Smile Dental\")"
}

### SeqTopV2 ###
{
 "input": "How long it will take me to get home from here if i leave now",
 "output": "GET_LOCATION_HOME() [SEP] GET_LOCATION(LOCATION_USER = \"here\") [SEP] GET_ESTIMATED_DURATION(DESTINATION = \"GET_LOCATION_HOME\"; SOURCE = \"GET_LOCATION\"; DATE_TIME_DEPARTURE = \"now\")"
}
\end{lstlisting}
\end{nolinenumbers}






\section{Instructions used for FineTuning}
Below is an example of our instruction data that is in input/output format. Where input combines the instruction, API specifications, and the Query.
\begin{nolinenumbers}
\begin{lstlisting}[language=json,firstnumber=1]
### SeqMultiWOZ ###
{
  "input": "Given the APIs and Slots below, sequence them in the order in which they have to be called to answer the following query. \n Possible APIs: book_hotel; book_restaurant; book_taxi; book_train; find_attraction; find_bus; find_hospital; find_hotel; find_restaurant; find_taxi; find_train; police \n Possible parameters: attraction-name; bus-departure; restaurant-bookday; restaurant-pricerange; hotel-pricerange; taxi-arriveby; bus-destination; taxi-departure; hotel-parking; hotel-area; hotel-type; bus-leaveat; hotel-bookpeople; hotel-bookday; train-departure; hotel-stars; train-bookpeople; restaurant-food; hospital-department; restaurant-area; restaurant-name; taxi-destination; hotel-internet; hotel-bookstay; attraction-type; taxi-leaveat; attraction-area; bus-day; train-arriveby; train-destination; train-day; restaurant-bookpeople; hotel-name; train-leaveat; police-name; restaurant-booktime \n Query: In the centre, there is a Japanese restaurant called Wagamama. It is expensive. book a restaurant in the centre called wagamama for 3 people at 12:15 on Saturday. It serves Japanese food and is expensive. Find a hotel with 2 stars and parking. \n Answer: ",
  "output": "find_restaurant(restaurant-area = \"centre\"; restaurant-food = \"japanese\"; restaurant-name = \"wagamama\"; restaurant-pricerange = \"expensive\") [SEP] book_restaurant(restaurant-area = \"centre\"; restaurant-bookday = \"saturday\"; restaurant-bookpeople = 3; restaurant-booktime = \"12:15\"; restaurant-food = \"japanese\"; restaurant-name = \"wagamama\"; restaurant-pricerange = \"expensive\") [SEP] find_hotel(hotel-parking = \"yes\"; hotel-stars = 2; hotel-type = \"hotel\")"
}
\end{lstlisting}
\end{nolinenumbers}

\begin{figure*}[hbt!]
\begin{center}
\includegraphics[width=0.8\textwidth]{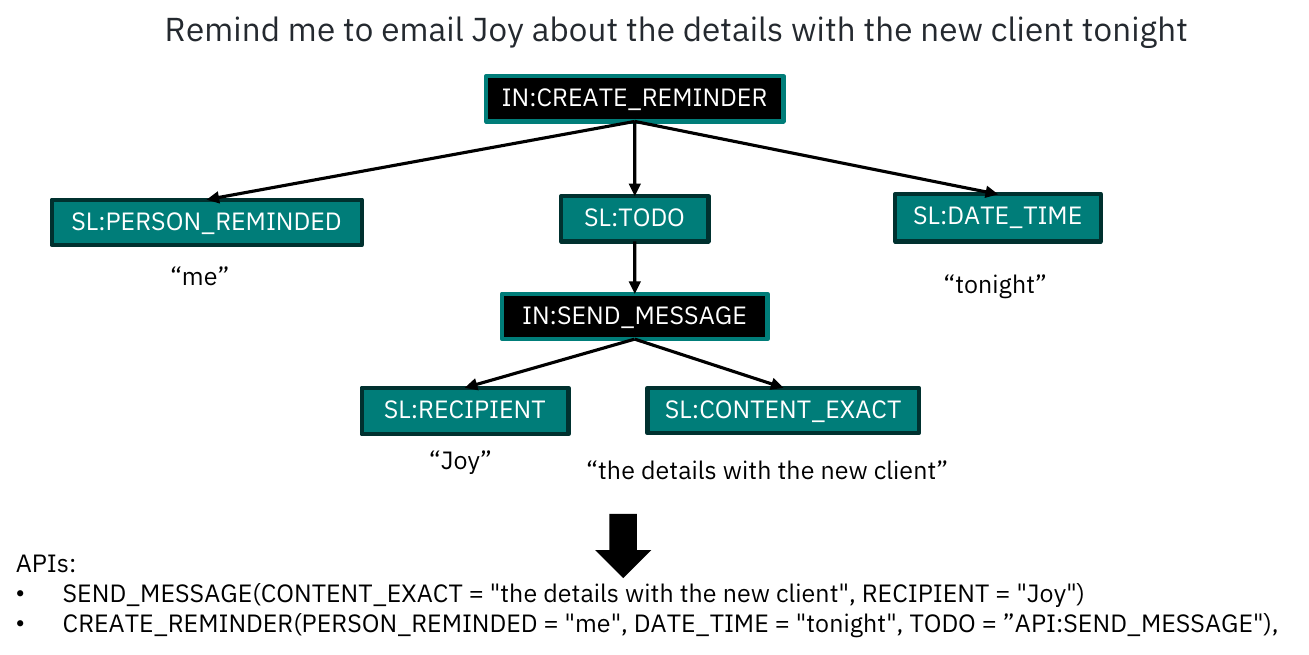}
\caption{Example of the creation process of SeqTopV2. Starting with the annotated semantic parse with mixed intents and slots, we convert it into a sequence of APIs. }
\label{topv2_ex}
\end{center}
\end{figure*}
